# Supplementary material for: The effect of spanwise heterogeneous surfaces on mixed convection in turbulent channels
Source: arXiv:2203.09817 source file (2022-08-08)
Supplement: Supplementary file 1 [file appendix.tex]

\section*{Statistics for discussion}

%###############################################################################
\begin{table}
    \begin{center}
    \begin{tabular}[b]{ccccccccc}
    $\mathrm{Ra}$ & $\mathrm{Re}_{b}$ & $\mathrm{Ri}_{b}$ & $S/\delta$ & $\delta_\textit{eff}/\delta$ & $\delta_\textit{eff}/L$  & $L$ & $\delta_\nu$ \\[3pt]
       \hline
      $0$    & 2800  & 0 & $\infty$ & 1     & - & - & 0.0056 \\
      $0$    & 2800  & 0 & 4        & 0.997 & - & - & 0.0055 \\
      $0$    & 2800  & 0 & 2        & 0.994 & - & - & 0.0055 \\
      $0$    & 2800  & 0 & 1        & 0.987 & - & - & 0.0054 \\
      $0$    & 2800  & 0 & 0.5      & 0.975 & - & - & 0.0050 \\[5pt]
      $10^5$ & 2800  & 0.003 & $\infty$ & 1     & 0.008 & 123.018 & 0.0055  \\
      $10^5$ & 2800  & 0.003 & 4        & 0.997 & 0.008 & 122.427 & 0.0055  \\
      $10^5$ & 2800  & 0.003 & 2        & 0.994 & 0.008 & 122.270 & 0.0055  \\
      $10^5$ & 2800  & 0.003 & 1        & 0.987 & 0.008 & 123.410 & 0.0053 \\
      $10^5$ & 2800  & 0.003 & 0.5      & 0.975 & 0.007 & 137.585 & 0.0050\\[5pt]
      %
      %$2.5\cdot10^5$ & 2800  & 0.008  & 1        & 0.987 & $512 \times 193\times 384$ & 8.895 & 185.2 & 8.196 & 0.020 & 3599 & 164\\[5pt]
      %
      $5.0\cdot10^5$ & 2800  & 0.016  & $\infty$ & 1     & 0.043 & 23.079 & 0.0055  \\
      $5.0\cdot10^5$ & 2800  & 0.016  & 4        & 0.997 & 0.042 & 23.706 & 0.0055 \\
      $5.0\cdot10^5$ & 2800  & 0.016  & 2        & 0.994 & 0.042 & 23.851 & 0.0054  \\
      $5.0\cdot10^5$ & 2800  & 0.016  & 1        & 0.987 & 0.041 & 24.260 & 0.0053  \\
      $5.0\cdot10^5$ & 2800  & 0.016  & 0.5      & 0.975 & 0.036 & 27.065 & 0.0049 \\[5pt]
      $7.5\cdot10^5$ & 2800  & 0.024  & $\infty$ & 1     & 0.075 & 13.835 & 0.0055 \\
      $7.5\cdot10^5$ & 2800  & 0.024  & 4        & 0.997 & 0.072 & 13.835 & 0.0055  \\
      $7.5\cdot10^5$ & 2800  & 0.024  & 2        & 0.994 & 0.069 & 14.384 & 0.0054 \\
      $7.5\cdot10^5$ & 2800  & 0.024  & 1        & 0.987 & 0.062 & 15.994 & 0.0053 \\
      $7.5\cdot10^5$ & 2800  & 0.024  & 0.5      & 0.975 & 0.055 & 17.888 & 0.0049 \\[5pt]
      $10^6$ & 2800  & 0.032 & $\infty$ & 1     & 0.106 & 9.438  & 0.0056  \\
      $10^6$ & 2800  & 0.032 & 4        & 0.997 & 0.103 & 9.710  & 0.0055  \\
      $10^6$ & 2800  & 0.032 & 2        & 0.994 & 0.099 & 10.000 & 0.0054  \\
      $10^6$ & 2800  & 0.032 & 1        & 0.987 & 0.092 & 10.677 & 0.0053  \\
      $10^6$ & 2800  & 0.032 & 0.5      & 0.975 & 0.079 & 12.272 & 0.0049 \\[5pt]
      $10^7$ & 0     & $\infty$ & $\infty$ & 1     & $\infty$ & -    & -   \\
      $10^7$ & 0     & $\infty$ & 4        & 0.997 & $\infty$ & -    & -  \\
      $10^7$ & 0     & $\infty$ & 2        & 0.994 & $\infty$ & -    & -   \\
      $10^7$ & 0     & $\infty$ & 1        & 0.987 & $\infty$ & -    & - \\
      $10^7$ & 0     & $\infty$ & 0.5      & 0.975 & $\infty$ & -    & -  \\[5pt]
      $10^7$ & 500   & 10.0  & $\infty$ & 1     & 24.357 & 0.041 & 0.0141   \\
      $10^7$ & 500   & 10.0  & 4        & 0.997 & 23.652 & 0.042 & 0.0138  \\
      $10^7$ & 500   & 10.0  & 2        & 0.994 & 23.033 & 0.043 & 0.0136   \\
      $10^7$ & 500   & 10.0  & 1        & 0.987 & 20.305 & 0.049 & 0.0127   \\
      $10^7$ & 500   & 10.0  & 0.5      & 0.975 & 18.188 & 0.054 & 0.0116  \\[5pt]
      $10^7$ & 1581  & 1.0 & $\infty$ & 1     & 3.079 & 0.325 & 0.0075   \\
      $10^7$ & 1581  & 1.0 & 4        & 0.997 & 2.960 & 0.337 & 0.0073  \\
      $10^7$ & 1581  & 1.0 & 2        & 0.994 & 2.850 & 0.349 & 0.0071 \\
      $10^7$ & 1581  & 1.0 & 1        & 0.987 & 2.679 & 0.369 & 0.0069  \\
      $10^7$ & 1581  & 1.0 & 0.5      & 0.975 & 2.447 & 0.399 & 0.0064  \\[5pt]
      $10^7$ & 2800  & 0.32 & $\infty$ & 1     & 1.116 & 0.896 & 0.0053    \\
      $10^7$ & 2800  & 0.32 & 4        & 0.997 & 1.085 & 0.919 & 0.0051   \\
      $10^7$ & 2800  & 0.32 & 2        & 0.994 & 1.056 & 0.941 & 0.0050    \\
      $10^7$ & 2800  & 0.32 & 1        & 0.987 & 1.002 & 0.986 & 0.0048  \\
      $10^7$ & 2800  & 0.32 & 0.5      & 0.975 & 0.931 & 1.047 & 0.0045 \\
    \end{tabular}
    \end{center}
\end{table}
\clearpage
%###############################################################################
\begin{table}
    \begin{center}
    \begin{tabular}[b]{ccccccccc}
    $\mathrm{Ra}$ & $\mathrm{Re}_{b}$ & $\mathrm{Ri}_{b}$ & $S/\delta$ & $\delta_\textit{eff}/\delta$ & $\delta_\textit{eff}/L$  & $L$ & $\delta_\nu$ \\[3pt]
       \hline
      $10^7$ & 5000  & 0.1 & $\infty$ & 1     & 0.379 & 2.640 & 0.0033  \\
      $10^7$ & 5000  & 0.1 & 4        & 0.997 & 0.376 & 2.654 & 0.0033 \\
      $10^7$ & 5000  & 0.1 & 2        & 0.994 & 0.366 & 2.717 & 0.0032  \\
      $10^7$ & 5000  & 0.1 & 1        & 0.987 & 0.357 & 2.763 & 0.0031  \\
      $10^7$ & 5000  & 0.1 & 1        & 0.975 & 0.338 & 2.881 & 0.0030 \\[5pt]
      $10^7$ & 10000 & 0.025  & $\infty$ & 1     & 0.106 & 9.476 & 0.0018   \\
      $10^7$ & 10000 & 0.025  & 4        & 0.997 & 0.102 & 9.707 & 0.0018   \\
      $10^7$ & 10000 & 0.025  & 2        & 0.994 & 0.102 & 9.759 & 0.0018    \\
      $10^7$ & 10000 & 0.025  & 1        & 0.987 & 0.095 & 10.433 & 0.0017   \\
      $10^7$ & 10000 & 0.025  & 0.5      & 0.975 & 0.084 & 11.550 & 0.0017  \\[5pt]
      $10^8$ & 2800  & 3.19 & $\infty$ & 1     & 10.743 & 0.093 & 0.0041  \\
      $10^8$ & 2800  & 3.19 & 4        & 0.997 & 10.816 & 0.092 & 0.0040 \\
      $10^8$ & 2800  & 3.19 & 2        & 0.994 &  9.910 & 0.100 & 0.0038 \\
      $10^8$ & 2800  & 3.19 & 1        & 0.987 &  9.403 & 0.105 & 0.0037  \\
      $10^8$ & 2800  & 3.19 & 0.5      & 0.975 &  8.193 & 0.119 & 0.0033 \\
      \hline
    \end{tabular}
    \caption{List of lengthscales.}
    \label{tbl:lengthscales}
    \end{center}
\end{table}

%######################################################
\section{Old summary}

The present work investigates the effect of heterogeneous rough surfaces on mixed convection in turbulent channel flow with unstable stratification by means of direct numerical simulations. 
%not only to vary the spatial extent of secondary motions in the forced convection regime but also to control the imposed drag on the flow.
The relative importance of buoyancy and shear effects are controlled by the bulk Richardson number $Ri_b$, which spans a large range of values for the present simulations to cover the different flow regimes forced, mixed and natural convection. 
%forced convection with dominant shear, mixed convection with equal contribution of shear and buoyancy and natural convection, which is purely driven by buoyancy effects.
The flow organisation of forced convection or weak buoyancy effects resembles the one from classical Poiseuille flow, while comparable contributions of shear and buoyancy in the mixed convection regime results in large-scale streamwise rolls.
For weak shear and strong buoyancy forces the flow organizes in convection cells similar to Rayleigh-Bénard flows \citep{Pirozzoli_mixed_2017}. 
The heterogeneous surface consists of streamwise-aligned Gaussian ridges, which are known to generate secondary motion in forced convection flows.
The spanwise spacing of the ridges $S$ controls the spatial extent of the secondary motion, seen in the time-averaged velocity fields, as well as the imposed drag on the flow \citep{hwang_secondary_2018}.
For the present simulation the ridge spacings is systematically varied from coarse to dense ridge spacings, to study its influence on the flow organisation in presence of buoyancy effects in the mixed and natural convection regime.

The results show that the introduction of Gaussian ridges leads to an increase of the skin friction drag $C_f$ compared to the smooth wall condition, not only for the pure forced convection case, but also for the mixed and natural convection cases. 
For all considered $Ri_b$ this increase intensifies as the ridge spacing $S$ becomes successively smaller. 
The heat transfer also increases for most cases, except for those with strong shear and weak buoyancy effects, which fall within a range of bulk Richardson number $Ri_b = 0.016-0.032$.
This range of Richardson numbers represents the transition at which flow structures from forced convection flow are replaced by streamwise rolls with increasing buoyancy effects, which occurs for the smooth wall case at $Ri_b=0.016$.
In contrast, this clear transition occurs in the case of ridges at higher buoyancy effects and is indicated by the disappearance of secondary motions.
The transition begins for the coarsest ridge spacing $S=4\delta$ at $Ri_b=0.016$ (still with some visible parts of secondary motion), and is completed at $Ri_b=0.032$ also for the two densest ridge spacings $S=\delta$ and $S=0.5\delta$.
Since denser ridge spacings introduce more drag and higher shear in the near-wall region, larger buoyancy forces are required to form streamwise rolls and thereby breaking the local symmetry of the secondary motions.

The organisation and formation of these streamwise rolls is strongly linked to low-speed streaks close to the wall \citep{khanna_ABL_1998}.
Within low-speed streaks localized buoyancy forces can concentrate and thereby create a linear updraft. 
Multiple updrafts can merge to a strong buoyancy-enhanced streak, which reaches the opposing wall and reduces or destroys the coherence of the low-speed streaks there. 
On the opposite wall and between these impingement region of the updrafts, buoyancy enhanced low-speed streaks are also formed, which in turn generate a strong localized downdraft and in combination result in a large-scale streamwise roll motion.
With increasing the relative importance of buoyancy to shear, this mechanism first intensifies the strength and coherence of the streamwise rolls, while for stronger buoyancy effects these rolls will eventually begin to merge and thereby forming convective cells \citep{Salesky_nature_2017}.
The maximum of this streamwise roll coherence, measured by the volume-averaged cross-sectional coherent kinetic energy, is found for the present simulation at $Ri_b = 1$, consistent with recent observation in ABL \citep{jayaraman_transition_2021}.
In presence of the Gaussian ridges it is found that warm-fluid and low-speed streaks are preferentially located at the ridges, which on the one hand supports the formation of the up- and downdrafts, while one the other hand it counteracts the up- and downdrafts in the impingement region at the opposite wall.

Interestingly, at the maximum of coherence at $Ri_b = 1$ the streamwise roll is very sensitive for the coarsest ridge spacing $S=4\delta$, which results in an almost complete destruction of the coherence of the roll, while for denser ridge spacings this reduction is less pronounced. 
Investigation of the mean velocity and temperature field in the cross-section reveal for this case, that the up- and downdraft region of the roll occur in the valley between adjacent ridges. 
Consequently, large horizontal lateral motion of the streamwise roll between the down- and updrafts will strike on the Gaussian ridge.
This introduces a recirculation zone at the lee side of the ridge and contributes to a strong lateral disturbance in the region of the updraft, thereby diminishing the organisation mechanism of the updraft (similar for $Ri_b=10$).
In contrast, the same ridge spacing $S=4\delta$ but slightly larger buoyancy forces $Ri_b=3.2$, leads to an increase in the coherence of the streamwise roll motion in comparison with the smooth wall condition. 
This is the only case where the up- and downdraft regions appear directly at the ridge position and due to the symmetric ridge configuration, impinge on an opposing ridge. 
This indicates, that the buoyancy forces in the up- and downdrafts are strong enough to reduce the influence of the low-speed streaks at the opposing ridge. 
As a result, the streamwise roll will not experience a ridge on their lateral horizontal movement, which leads to a reduced increase of $C_f$ compared to case $Ri_b=1$ with the same ridge spacing.
(Why does the coherence goes down again for $Ri_b = 10$ and $S=4\delta$? Probably a Reynolds number effect, since the viscous length is larger than for $Ri_b = 3.2$ the low-speed streaks have larger wall-normal extent, and probably are able to counteract the up-downdrafts again...)

Results of secondary motion with a staggered arrangement of the ridges at opposing wall were found to increase the coherence of the secondary motion, and we thus speculate, that without an opposing ridge at the up- and downdraft region, the coherence would be even stronger for the streamwise roll \citep{stroh_secondary_2020}.

In general, for the streamwise roll regime and dense ridge spacings ($S \le 2\delta$) a reduction of $S$ leads to a monotonic decrease of the coherence of the streamwise rolls compared to the smooth wall case.
For the moderate convective cases $Ri_b =3.2$ and $Ri_b = 10$ the densest ridge spacing $S=0.5\delta$ reduces the coherence that strong, such that the streamwise rolls are replaced by convection cells.
In the ABL community it is an ongoing discussion whether there is a coexistence of rolls and cells within this stability parameter range \cite{Salesky_nature_2017}.
Here, we can clearly see, that a sufficient strong drag imposed by the densely spaced ridges is already sufficient to trigger convection cells at relatively low stability parameters.
The convection cells found for these two cases have a preferred orientation perpendicular to the aligned ridges.
This is also found for the two densest ridge spacings of the purely natural convection case.
While the natural convection case with smooth wall conditions has no preferential orientation of the cell (only a slight imbalance of $\langle\overline{u'u'}\rangle$ and $\langle\overline{w'w'}\rangle$, which is likely due to the non quadratic horizontal domain size), the introduction of ridges and the successive decrease of the ridge spacing lead to increasingly preference of the cells to orient perpendicular to the ridges. 
Similar, as for the streamwise rolls, the lateral near-wall motion of the convection cell is increasingly disturbed by denser ridge spacings, such that the flow of the cell prefers to stream along the aligned ridges.

The present results show that heterogeneous roughness in form of aligned Gaussian ridges can have a significant influence of the flow organization in mixed convection. 
The transition between forced convection structures to streamwise roll is altered by the presence of ridges towards larger bulk Richardson number, which indicates that the increased shear by the ridges requires larger buoyancy forces to form streamwise rolls.
Especially, for the moderate convective conditions, the roughness triggers the transition from streamwise rolls to convection cells, than expected for smooth wall conditions. 
As such the range where streamwise rolls appear over smooth walls is significantly reduced by the heterogeneous roughness. 
Overall, this suggest that roughness effects can be equally important for the flow organization as a change of magnitude of the $Ri_b$.
This has strong implications for the parametrization of the dynamics of the ABL of the weather and climate models, which might influence the distribution of water vapour (clouds?), dust, pollutants.
